# Supplementary material for: Mid-Infrared Optical Spin Injection and Coherent Control
Source: arXiv:2212.04472 ancillary file (2022-12-08)
Supplement: Supplementary file 1 [file Supporting_information.pdf]

# Supplementary Material: Mid-Infrared Optical Spin Injection and Coherent Control

G. Fettu,[1] J. E. Sipe,[2] and O. Moutanabbir[1]

[1] *Department of Engineering Physics, École Polytechnique de Montréal, C.P. 6079, Succ. Centre-Ville, Montréal, Québec, Canada H3C 3A7*

[2] *Department of Physics and Institute for Optical Sciences, University of Toronto, 60 St. George Street, Toronto, Ontario, Canada M5S 1A7*

## CONTENTS

I. Two-photon absorption 1
A. Two-photon carrier injection 1
B. Two-photon spin injection 1

II. Coherent control 2
A. Colinearly polarized beams configuration 2
B. Circularly polarized beams configuration 2

References 3

## I. TWO-PHOTON ABSORPTION

The spectral dependence of two-photon carrier and spin injection processes in $Ge_{1-x}Sn_x$ can be analyzed by calculating the associated tensors over a range of energies. By symmetry of the diamond structure, the fourth-rank carrier injection tensor $\xi_2^{abcd}$ has 3 independent components, while the fifth-rank spin injection pseudotensor $\zeta_2^{abcde}$ has 2 independent components. For each quantity, one independent component is presented in the main article; the others are shown in the present document.

### A. Two-photon carrier injection

The expression for the fourth-rank tensor associated to two-photon carrier injection is:

$$\xi_2^{abcd}(\omega) = \frac{2\pi e^4}{\hbar^4\omega^4}\sum_{c,v}\int \frac{\mathrm{d}^3k}{8\pi^3} w_{cv}^{ab*}(\mathbf{k}) w_{cv}^{cd}(\mathbf{k})\delta\left[\omega_{cv}(\mathbf{k}) - 2\omega\right] \quad (1)$$

where $\boldsymbol{w}_{cv}^{ab}(\mathbf{k})$ is the symmetrized two-photon amplitude:

$$w_{cv}^{ab}(\mathbf{k}) \equiv \frac{1}{2}\sum_m \frac{v_{cm}^a(\mathbf{k})v_{mv}^b(\mathbf{k}) + v_{cm}^b(\mathbf{k})v_{mv}^a(\mathbf{k})}{\omega_m(\mathbf{k}) - \bar{\omega}_{cv}(\mathbf{k})}. \quad (2)$$

In the main text, the independent component $\xi_2^{xxxx}$ is presented. In Fig. 1 and Fig. 2, the independent components $\xi_2^{xxyy}$ and $\xi_2^{xyxy}$ are shown, respectively. Within the independent particle approximation, they are purely real, and associated to the third-order nonlinear susceptibility $\boldsymbol{\chi}^{(3)}$ by $\mathrm{Im}\left[\chi^{(3)}(\omega;-\omega,\omega,\omega)\right] = (\hbar/3)\xi_2(\omega)$.

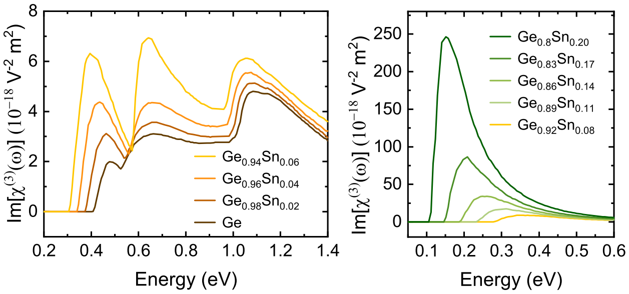


FIG. 1. The component $\xi_2^{xxyy}$ of the two-photon absorption tensor $\xi_2(\omega)$ in $Ge_{1-x}Sn_x$, as a function of photon energy $\hbar\omega$, at various Sn compositions from 0 to 20%.

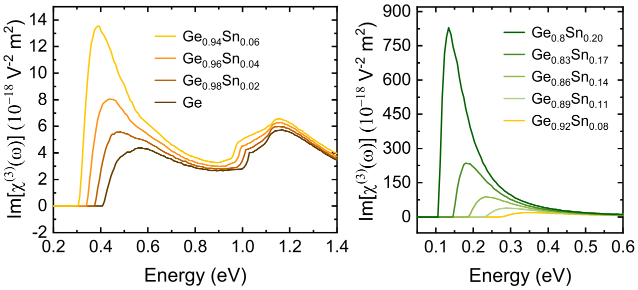


FIG. 2. The component $\xi_2^{xyxy}$ of the two-photon absorption tensor $\xi_2(\omega)$ in $Ge_{1-x}Sn_x$, as a function of photon energy $\hbar\omega$, at various Sn compositions from 0 to 20%.

Similarly to $\xi_2^{xxxx}$, in addition to the expected direct band gap energy reduction, the two other components exhibit a surge in magnitude close to the band edge, when the Sn content increases. This surge is almost exponential relatively to the Sn content, and can be attributed to a reduction of the carrier effective masses. The $xxyy$ component is particularly sensitive to the onset of absorption from the split-off band, at around 0.6 eV, contrary to the $xyxy$ component.

### B. Two-photon spin injection

The two-photon spin injection processes are associated to the fifth-rank pseudotensor $\zeta_2^{abcde}$. In the main article, the independent component $\zeta_2^{xxyxz}$ is presented, and in Fig. 3, the other independent component $\zeta_2^{xyzzz}$ is shown. They are purely imaginary within the single-particle approximation. The expression for the pseudotensor is:

$$\zeta^{abcde}_{\substack{2;e\\(h)}}(\omega) = (-)\frac{\pi e^4}{\hbar^4\omega^4}\sum_{\substack{c,c',v\\(c,v,v')}}^{\prime}\int\frac{d^3k}{8\pi^3}S^a_{\substack{cc'\\(v'v)}}(\mathbf{k})w^{bc*}_{cv}(\mathbf{k})w^{de}_{\substack{c'v\\(cv')}}(\mathbf{k})$$
$$\times\left(\delta\left[\omega_{cv}(\mathbf{k})-2\omega\right]+\delta\left[\omega_{\substack{c'v\\(cv')}}(\mathbf{k})-2\omega\right]\right). \quad (3)$$

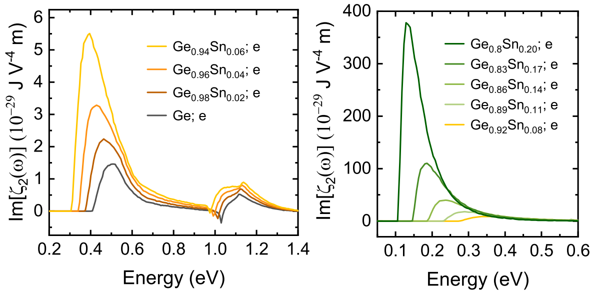


FIG. 3. The electron contribution to the component $\zeta_2^{xyzzz}$ of the two-photon spin injection pseudotensor $\zeta_2(\omega)$ in $\mathrm{Ge}_{1-x}\mathrm{Sn}_x$, as a function of photon energy $\hbar\omega$. The different curves show various Sn composition of the alloy, from 0 to 20%.

The component $xyzzz$ shows very similar features compared to the component $xxyxz$ presented in the main article. Close to the band edge, there is a strong augmentation of two-photon spin injection when the Sn content increases. At the $E_1$ transition, there is a slight broadening of the peak. The overall magnitude of this component is lower than the other independent one.

## II. COHERENT CONTROL

There are three main polarization configurations for coherent control within the two-color scheme: colinear polarizations, cross-linear polarizations and circularly polarized beams. In this section, the swarm velocity of the charge current in the case of colinear polarizations is presented. Additionally, the interference charge and spin current calculations for circularly polarized beams are shown.

### A. Colinearly polarized beams configuration

In the colinear polarization configuration, a strong charge current proportional to the tensor component $\eta_I^{xxxx}$ is generated. The spectral dependence of this component is presented in the main article. The swarm velocity is a measure of the average velocity per injected carriers, and is defined by:

$$v_s^x = \frac{\dot{J}^x}{e\dot{n}} \quad (4)$$

with $\dot{n}$ the total injection rate for carrier density, $\dot{J}^x$ the charge current injection, and $e$ the electronic charge. The maximal value of the swarm velocity, as defined in Ref. [1], is given by:

$$v^x_{\mathrm{s,max}}(\omega) = \frac{Im[\eta_I^{xxxx}(\omega)]}{e\sqrt{\xi_1^{xx}(2\omega)\xi_2^{xxxx}(\omega)}}. \quad (5)$$

The results of the calculations for $v^x_{\mathrm{s,max}}$ in $\mathrm{Ge}_{1-x}\mathrm{Sn}_x$, for various alloy compositions, are shown in Fig. 4.

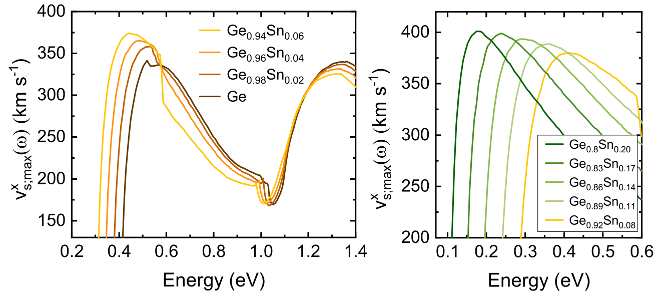


FIG. 4. Maximal swarm velocity $v^x_{\mathrm{s,max}}$ for the charge current injected in $\mathrm{Ge}_{1-x}\mathrm{Sn}_x$ with colinearly polarized $\omega$ and $2\omega$ beams. The different curves show various Sn composition of the alloy, from 0 to 20%.

As the Sn content increases, the maximal swarm velocity increases close to the band edge, and reaches 400 $km/s$ for 20% of Sn. In the 0.6eV-1eV range, the drop in velocity is even more prominent for Sn content up to 6%, compared to pure Ge.

### B. Circularly polarized beams configuration

The charge current and spin current injected in the case of circularly polarized beams, are described respectively by the following equations:

$$\dot{\mathbf{J}}_I = \frac{1}{\sqrt{2}}\,\mathrm{Im}\left[\eta_I^{xxxx}-\eta_I^{xyyx}+2\eta_I^{xxyy}\right]E_\omega^2E_{2\omega}\hat{\mathbf{m}}, \quad (6)$$

$$\dot{K}_I^{ab} = \pm\frac{1}{\sqrt{2}}\left(\mu_I^{xyzzz}-\mu_I^{xyxxz}+2\mu_I^{xyzxz}\right)E_\omega^2E_{2\omega}\hat{\mathbf{m}}^a\hat{\mathbf{z}}^b$$
$$\mp\frac{1}{\sqrt{2}}\left(\mu_I^{xyzzz}-\mu_I^{xyyyz}+2\mu_I^{xyyzy}\right)E_\omega^2E_{2\omega}\hat{\mathbf{z}}^a\hat{\mathbf{m}}^b, \quad (7)$$

where $\hat{\mathbf{m}} = \hat{\mathbf{x}}\sin(\Delta\phi) \pm \hat{\mathbf{y}}\cos(\Delta\phi)$.

In Fig. 5, the results of Eq. (6) (including the $\frac{1}{\sqrt{2}}$ factor, but excluding the terms related to the optical fields) in $\mathrm{Ge}_{1-x}\mathrm{Sn}_x$ are presented. These are similar than the results obtained for the component $\eta_I^{xxxx}$, presented in

the main article. Indeed, close to the band edge, there is a strong augmentation of the magnitude of charge current injection as the Sn content increases. It can be explained by the reduction of the electron effective mass in the material.

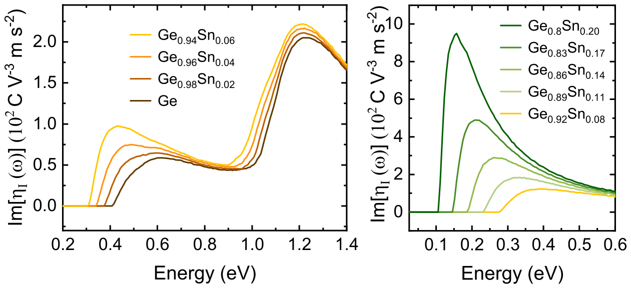


FIG. 5. The electron contribution to the charge current injection tensor, associated to circularly polarized beams in $Ge_{1-x}Sn_x$, as a function of photon energy $\hbar\omega$. The different curves show the evolution at various Sn compositions from 0 to 20%.

In Fig. 6, the results of the first line of Eq. (7) (including the $\frac{1}{\sqrt{2}}$ factor, but excluding the terms related to the optical fields) in $Ge_{1-x}Sn_x$ are presented.

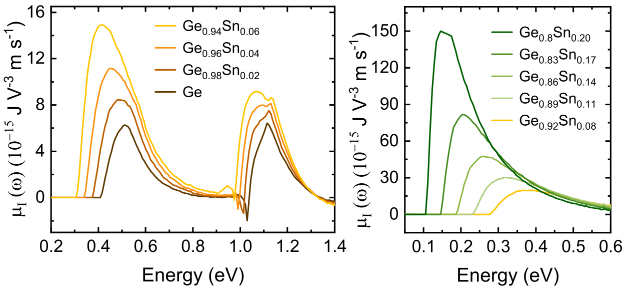


FIG. 6. The electron contribution to the spin current injection pseudotensor, associated to circularly polarized beams in $Ge_{1-x}Sn_x$, as a function of photon energy $\hbar\omega$. The different curves show various Sn composition of the alloy, from 0 to 20%.

The features are analogous to the independent component $\mu_I^{xyxxz}$ presented in the main article, with a peak close to the band edge and a second one at energies corresponding to the $E_1$ transition. With the incorporation of Sn in Ge, both these peaks grow significantly, particularly the one close to the direct gap.

[1] J. Rioux and J. Sipe, Physical Review B **81**, 155215 (2010).
